# Supplementary material for: Quantum Nonlinear Optics with a Germanium-Vacancy Color Center in a Nanoscale Diamond Waveguide
Source: arXiv:1612.03036 ancillary file (2017-06-01)
Supplement: Supplementary file 1 [file GeV_waveguide_SI.pdf]

# Supplemental Material: Quantum Nonlinear Optics with a Germanium-Vacancy Color Center in a Nanoscale Diamond Waveguide

M. K. Bhaskar,[1,*] D. D. Sukachev,[1,2] A. Sipahigil,[1] R. E. Evans,[1] M. J. Burek,[3] C. T. Nguyen,[1] L. J. Rogers,[4] P. Siyushev,[4] M. H. Metsch,[4] H. Park,[5] F. Jelezko,[4] M. Loncar,[3] and M. D. Lukin[1,†]

[1]*Department of Physics, Harvard University, 17 Oxford Street, Cambridge, Massachusetts 02138, USA*
[2]*P. N. Lebedev Physical Institute of the RAS, Moscow 119991, Russia*
[3]*John A. Paulson School of Engineering and Applied Sciences, Harvard University, 29 Oxford Street, Cambridge, Massachusetts 02138, USA*
[4]*Institute for Quantum Optics, University Ulm, Albert-Einstein-Allee 11, 89081 Ulm, Germany*
[5]*Department of Chemistry and Chemical Biology, Harvard University, 12 Oxford St., Cambridge, Massachusetts 02138, USA*

## I. EXPERIMENTAL SETUP

All experiments at $T = 5\,\mathrm{K}$ are performed in a modified liquid helium flow probe-station (Desert Cryogenics model TTP4). We use a dual-axis scanning galvonometer mirror system (Thorlabs GVS012) and a high NA objective (Olympus 100x 0.90 NA) to deliver light via free-space in the experiments presented in Fig. 1-4, S1 [S1]. We use a $520\,\mathrm{nm}$ diode laser (Thorlabs LP520-SF15) for off-resonant continuous-wave excitation [Fig. 1(b) and Fig. 2(c)] and a pulsed $532\,\mathrm{nm}$ laser (PicoQuant PDL 800-B) to perform lifetime measurements [Fig. 2(d) and Fig. S1]. We employ sum-frequency generation using a nonlinear crystal (ADVR KTP), mixing $\sim 980\,\mathrm{nm}$ laser light from a Ti:Sapphire laser (M-Squared SolsTiS-2000-PSX-XF) and $1550\,\mathrm{nm}$ laser light from an external cavity diode laser (Thorlabs SFL 1550P) in a fiber-based wavelength division multiplexer (Thorlabs WD202A-APC). The output fiber is cleaved and coupled to a waveguide in the nonlinear crystal, which has $\sim 1\,\mathrm{nm}$ bandwidth. We tune the frequency of the Ti:Sapphire laser to modulate the frequency of the $\sim 600\,\mathrm{nm}$ light. The wavelength is recorded on a high resolution wavemeter (High Finesse WS7) with $10\,\mathrm{MHz}$ resolution and $50\,\mathrm{MHz}$ accuracy.

GeV centers are incorporated into devices at low density using $^{74}\mathrm{Ge}^{+}$ ion implantation (Innovion Corporation, $10^9$ $\mathrm{Ge}^{+}/\mathrm{cm}^2$ at an energy of $275\,\mathrm{keV}$) and subsequent high temperature annealing at $1200\,^{\circ}\mathrm{C}$ in vacuum. Waveguides are oriented along the $\langle 110 \rangle$ axis of the diamond. Confocal microscopy is used to collect light in the experiments presented in Fig. 1(b), Fig. 2(d), and Fig. S1. In all other experiments, light in the waveguide is collected using a tapered optical fiber [S2]. Technical details on fiber coupling and calibration of coupling efficiency are given in the supplementary materials of [S1]. Single photons are detected on an avalanche-photodiode (APD - Excelitas SPCM-ARQH).

* mbhaskar@g.harvard.edu
† lukin@physics.harvard.edu

## II. GEV-WAVEGUIDE COUPLING EFFICIENCY

We define the GeV-waveguide coupling efficiency $\beta$ as the probability for the GeV to emit a photon into the waveguide mode per excitation. To estimate $\beta$, we measure the saturation of ZPL fluorescence from a single GeV center in a waveguide [Fig. 2(b)]. We fit to a two-level model of saturation $D = D_{max} I/(I + I_{sat})$ where $D$ and $D_{max}$ are the detected and maximum possible detected intensities respectively, and $I$ and $I_{sat}$ are the applied and saturation intensities respectively. This predicts a maximum detected count rate of $D_{max} = 0.79 \pm .02$ Mcps.

Since we filter for ZPL photons (Semrock FF01-605/15-25), we collect roughly $60\%$ of the total emission spectrum given by the ZPL branching ratio [S3]. We only collect the photons emitted into the direction of the tapered fiber, resulting in another factor of $0.5$. Next we account for coupling to the tapered fiber ($\sim 0.5$), transmission through two 90:10 beamsplitters (Thorlabs TW670R2A2) in the fiber network ($\sim 0.8$), and re-collimation into fiber after a spectral filter (Semrock TLP01-628-25x36, free space-fiber coupling efficiency $\sim 0.8$). We send the light to an APD which has detector quantum efficiency $\sim 0.6$ at $\lambda = 600\,\mathrm{nm}$.

The maximum single-photon detection rate is given by one photon per excited state lifetime ($6.6 \pm 0.3$ ns), yielding a rate of about $160$ Mcps. Accounting for all of the factors described above, we expect a count rate of $\sim 8$ Mcps assuming the GeV emits every photon into the waveguide mode. From the maximum detection rate $\sim 0.8$ Mcps, we can place a lower bound on the probability of emission into the waveguide $\beta \geq 0.1$.

This is lower than the simulated value for $\beta$ in the designed nanostructure, which is roughly $0.7$ (Lumerical). The angle of the GeV dipole with respect to the waveguide and improper placement of the GeV with respect to the waveguide mode maximum likely limit the GeV-waveguide coupling in this experiment. We also note that this is a lower bound for $\beta$, since we do not account for time spent in unknown dark states such as different charge states of the GeV center.

## III. LINEWIDTH MEASUREMENTS

In Fig. 3(a) we measure the linewidth of transition 1-3 [Fig. 1(b)] at $T = 5\,\mathrm{K}$ for a single GeV in a waveguide using photo-

luminescence excitation (PLE) spectroscopy. The frequency of the excitation laser is scanned over the resonance several times, and fluorescence in the phonon sideband (PSB) is sent to an APD. We sum the different line-scans without correcting for background or spectral diffusion shifts of the line-position. We fit a Lorentzian to the integrated data in the main text and find a full-width at half maximum of $\gamma/(2\pi) = 72.8 \pm 1.4$ MHz, where the error given is the fit error to the data.

We note that the measurement of narrow GeV resonances in waveguides is not limited to this single GeV center. For a total of 6 different GeV centers in waveguides, we observe an average linewidth of $100 \pm 28$ MHz at $T = 5\,\text{K}$. While further work is needed to establish reliable statistics for GeV linewidths, these results demonstrate the reproducibility of narrow GeV optical transitions in nanostructures. Additionaly, PLE spectroscopy of GeV centers in bulk diamond at $T = 2.2\,\text{K}$, carried out in [S4], demonstrates a narrow 42 MHz line that is stable over long timescales.

We measure the excited state lifetime to extract the lifetime-limited linewidth for the GeV center described in the main text using pulsed off-resonant $532\,\text{nm}$ excitation. We record the decay of ZPL fluorescence in the time-domain using fast acquisition electronics (PicoQuant HydraHarp 400) and fit to a bi-exponential model that accounts for the sharp background from the strong laser pulse with the first exponent, and the lifetime of the GeV excited state with the second exponent. This is the same technique used to determine GeV lifetimes in Fig. 2(d). For this GeV, we measure a lifetime $\tau_0 = 6.1 \pm 0.2$ ns, shown in Fig. S1. From this measurement we extract a lifetime-broadened linewidth of $\gamma_0/(2\pi) = 26 \pm 1$ MHz.

We probe the contribution of phonon relaxation between orbital sublevels to the optical transition linewidth of several GeV centers for temperatures between $T = 35\,\text{K}$ and $T = 350\,\text{K}$ [Fig. 3(a) inset] using off-resonant $520\,\text{nm}$ excitation and recording the linewidth on a spectrometer (Horiba iHR550 with Synapse CCD and 1800 gr/mm, resolution $0.025\,\text{nm}$). The transition linewidth scales as $T^3$ (see main text for fit details). The $T^3$ fit implies that a two-phonon process is the dominant broadening mechanism at $T > 50\,\text{K}$, similar to the case of the SiV [S5]. We note that at temperatures $T > 100\,\text{K}$, the line is too broad to resolve the fine structure exactly, and we measure collective features from transitions C and D. For $T > 200\,\text{K}$, all four lines merge to give one linewidth. These imperfections only modify the measured linewidth by a small multiplicative factor, and the $T^3$ fit remains effective.

## IV. OPTICAL RABI OSCILLATION MEASUREMENTS

In order to probe optical relaxation dynamics at higher resonant excitation intensities, we utilize an active preselection sequence. We first probe the resonance with a weak resonant pulse, and detect scattered PSB photons on an APD. Using a fast counter on a field-programmable gate-array (Lattice Diamond MachX02HE), we determine if the GeV satisfies the resonance condition based on whether or not the GeV scatters more photons than a user-defined threshold. If the GeV is not

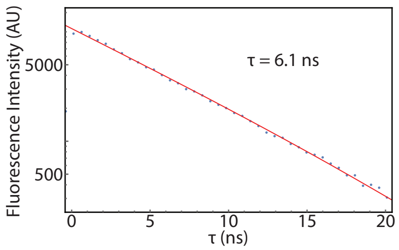


FIG. S1. Lifetime measurement of the GeV used for Fig. 3-5 in the main text. Pulsed $532\,\text{nm}$ excitation is applied. ZPL fluorescence is plotted on a log scale as a function of time $\tau$ from pulse leading edge.

on resonance, we apply a strong $520\,\text{nm}$ pulse which further speeds up spectral diffusion, randomizing the resonance position. We then repeat the procedure until the GeV scatters the threshold number of photons and is determined to be on resonance. By optimizing the power and duration of the various pulses as well as the photon detection threshold, we can maintain an experimental duty cycle of $\sim 50\%$ while remaining on resonance.

We utilize this sequence to measure optical Rabi oscillations with the same GeV center described in the PLE measurement in Fig. 3(a). Once we determine that the GeV is on resonance, we apply a strong $40\,\text{ns}$ resonant pulse and measure the fluorescence on the PSB in the time-domain [Fig. 3(b)] using fast acquisition electronics. We fit to the data using a two-level model of exponentially decaying oscillations of the form $(g/2)\Theta(t-t_0)(1-\mathcal{C}\exp(-|t-t_0|/\tau_{Rabi})\cos(2\pi\Omega(t-a)))$. Here $g$ is an amplitude normalization factor, $\Theta(t-t_0)$ is a step function at a time $t = t_0$ of the pulse leading edge, $\mathcal{C}$ is the contrast of Rabi oscillations, $\tau_{Rabi}$ is the decay constant of Rabi oscillations, and $\Omega$ is the Rabi frequency. For the measurement shown in the main text, we obtain $\mathcal{C} = 0.71 \pm 0.03$, $\Omega = 310 \pm 2$ MHz, and $\tau_{Rabi} = 6.59 \pm 0.02$ ns.

We repeat this measurement and fitting protocol at various temperatures up to $T = 10\,\text{K}$, at which point the Rabi oscillations decay too fast to resolve and fit effectively. We measure $\tau_{Rabi}$ as a function of temperature and plot the Rabi oscillation decay rate $\gamma_{Rabi}/(2\pi) = 1/(2\pi\tau_{Rabi})$ as a function of temperature [Fig. 3(b) inset]. At low temperatures ($T < 10\,\text{K}$) the decay rate of Rabi oscillations scales linearly with temperature. We fit to a linear model $\gamma_{Rabi}/(2\pi) = h + kT$ and obtain $h = -7.0 \pm 1.3$ MHz, and $k = 6.6 \pm 0.2$ MHz/K. The linear dependence of Rabi oscillation decay indicates that the transition is primarily broadened by a single phonon process at low temperatures between $T = 5\,\text{K}$ and $T = 10\,\text{K}$, again similar to the case of the SiV [S5].

For all temperature measurements, temperature is measured using a diode (Lakeshore DT-670A-CU) mounted to the sample holder. As a result, we do not probe the local temperature of the diamond nanostructure, potentially resulting in a small systematic temperature shift ($\sim 1\,\text{K}$) for all reported values. We note that this does not influence the linear and cubic scal-

ings of Rabi oscillation decay and linewidth at low and high temperatures respectively.

## V. GEV-WAVEGUIDE COOPERATIVITY

We calculate the cooperativity using the measured extinction in Fig. 4(b) following [S6]. The measurement is taken at $I/I_{sat} \sim 0.02$, satisfying the condition for low power ($\Omega_c/\Gamma \ll 1$ in [S6]). In this limit, the transmitted intensity on resonance ($\mathcal{T}$) is related to the cooperativity by $\mathcal{T} \approx (1+C)^{-2}$. We fit a Lorentzian to the transmission data to extract a measured extinction of $18 \pm 1\%$, corresponding to $\mathcal{T} = 0.82 \pm 0.01$, yielding a cooperativity of $C = 0.10 \pm 0.01$, as reported in the main text.

We note that this is a lower bound on the cooperativity, since this formula for cooperativity is for a two-level system. Finite thermal occupation of the upper branch of the ground state [state 2 in Fig. 1(b)] reduces the measured extinction. One can approach the expected extinction of a two level system by polarizing the system in state 1 using optical pumping [S1]. The presence of additional levels also reduces the measured extinction due to the branching ratios of different transitions (e.g. transition 2-3 and the PSB). Line-broadening mechanisms discussed above also reduce the system cooperativity. Furthermore, the same factors limiting the waveguide-GeV coupling $\beta$ also limit the cooperativity in this experiment.

The quantum efficiency, $QE$, is defined as the ratio of the radiative decay $\gamma_{rad}$, to the total excited state decay $\gamma_0$ [S7]. Because $\Gamma_{1D} < \gamma_{rad}$ and $\gamma_0 < \Gamma'$ due to the ZPL branching ratio and line-broadening, the cooperativity naturally places a lower bound on the quantum efficiency: $C = \Gamma_{1D}/\Gamma' < \gamma_{rad}/\gamma_0 = QE$. From the measurement in Fig. 4(b), we extract $C > 0.1$. Accounting for additional measured factors that reduce the cooperativity, but not the quantum efficiency, such as line-broadening beyond the lifetime limit ($26\,\mathrm{MHz}/73\,\mathrm{MHz} \sim 0.4$) and the branching ratio into the ZPL ($\sim 0.6$), we can place a tighter lower bound on the quantum efficiency $QE > 0.4$.

## VI. HOMODYNE MEASUREMENT

In this measurement, we excite through one port of a $90:10$ beamsplitter connected to the tapered fiber, sending $10\%$ of the near resonant excitation laser light to the diamond waveguide. We collect light through the fiber on the adjacent $90\%$ port of the beamsplitter. The detected ZPL field consists of interference between two fields: a local oscillator field $\mathbf{E}_{LO}$ arising from partial reflection of the driving laser from the Bragg mirror and resonance fluorescence $\mathbf{E}_{RF}$ stimulated by the driving field.

The diamond waveguide has two orthogonal polarization modes (TE and TM) [S8], which in principle can be treated independently. We neglect higher order waveguide modes which couple weakly to the fiber. The relative weights between $\mathbf{E}_{RF}$ and $\mathbf{E}_{LO}$ will differ for the two modes depending on their projections onto GeV dipole axis and the reflectivities of TE and TM fields from the Bragg mirror. The relative phases between the fields will also differ for TE and TM inputs due to the difference in waveguide group velocity for the TE and TM modes, allowing us to vary the phase by changing the input polarization.

Instead of treating the two modes separately, we consider an intuitive single-mode interference picture where $E_{RF} = \alpha S(\Delta) E_{LO} e^{i\phi}$. Here $\alpha$ and $\phi$ are free parameters that characterize the relative weight and phase of the two fields. $S(\Delta) = (1 - 2i\Delta/\gamma)^{-1}$ accounts for the Lorentzian resonance fluorescence spectrum for a given drive detuning $\Delta$ and transition full-width $\gamma$. In this model, the detected intensity is proportional to $|1 + \alpha S(\Delta) e^{i\phi}|^2$. We fit this model to the data presented in Fig. 5(b) of the main text leaving $\alpha$ and $\phi$ as free, continuous parameters ($\alpha \in [0,1]$ and $\phi \in [0, 2\pi)$). Using this technique, we determine relative phases $\phi = (0.98 \pm 0.02)\pi$ for the absorptive profile (orange) and $\phi = (1.66 \pm 0.01)\pi$ for the dispersive profile (blue). Intuitively, a relative phase of $\pi$ ($3\pi/2$) produces the typical absorptive (dispersive) Lorentzian lineshape evident in the measured interference spectrum.

We note that the single-mode model is an incomplete description of the homodyne measurement. We treat the problem of single-mode interference with a tunable relative phase because the two-mode problem introduces several additional free-parameters, and the single-mode picture captures the essential interference phenomenon present in the homodyne measurement. Additionally, there exist higher order terms resulting from interactions between the reflected field and the GeV center, as well as GeV self-interaction arising from the mirror. These terms are suppressed by the mirror reflectivity $R < 0.25$ and can in principle be incorporated into the model by redefining $\alpha$ and $\phi$. We neglect these higher order terms to preserve the simple physical interpretations of $\alpha$ and $\phi$ as the relative weight and phase between two fields.

To demonstrate the single-photon nonlinearity, we measure the photon statistics of the output field under a drive field with polarization that produces destructive interference ($\phi \sim \pi$). We split the output field on a $50:50$ beamsplitter and measure time dependent correlations using fast acquisition electronics. The total acquisition time for this measurement was $\sim 5$ hours. We postselect coincidence events that occur within 10 ms intervals for which the detected intensity is below $15\%$ of the steady state detuned value, ensuring that we include only data for which the drive field is nearly resonant with the GeV center ($\sim 25\%$ duty cycle). We fit to the data using a single exponential of the form $1 + he^{-t/\tau_b}$ to obtain the reported bunching $g^{(2)}(0) = 1 + h = 1.09 \pm 0.03$ decaying on a timescale $\tau_b = 6.2 \pm 2.7$ ns, close to the GeV excited state lifetime.

[S1] A. Sipahigil, R. E. Evans, D. D. Sukachev, M. J. Burek, J. Borregaard, M. K. Bhaskar, C. T. Nguyen, J. L. Pacheco, H. A. Atikian, C. Meuwly, *et al.*, Science **354**, 847 (2016).
[S2] M. J. Burek, C. Meuwly, R. E. Evans, M. K. Bhaskar, A. Sipahigil, S. Meesala, D. D. Sukachev, C. T. Nguyen, J. L. Pacheco, E. Bielejec, *et al.*, arXiv preprint arXiv:1612.05285 (2016).
[S3] Y. N. Palyanov, I. N. Kupriyanov, Y. M. Borzdov, and N. V. Surovtsev, Sci. Rep. **5**, 14789 (2015).
[S4] P. Siyushev, M. H. Metsch, A. Ijaz, J. M. Binder, M. K. Bhaskar, D. D. Sukachev, A. Sipahigil, R. E. Evans, C. T. Nguyen, M. D. Lukin, *et al.*, arXiv preprint arXiv:1612.02947 (2016).
[S5] K. D. Jahnke, A. Sipahigil, J. M. Binder, M. W. Doherty, M. Metsch, L. J. Rogers, N. B. Manson, M. D. Lukin, and F. Jelezko, New J. Phys. **17**, 043011 (2015).
[S6] D. E. Chang, A. S. Sørensen, E. A. Demler, and M. D. Lukin, Nat. Phys. **3**, 807 (2007).
[S7] R. N. Patel, T. Schröder, N. Wan, L. Li, S. L. Mouradian, E. H. Chen, and D. R. Englund, Light Sci. Appl. **5**, e16032 (2016).
[S8] M. J. Burek, Y. Chu, M. S. Liddy, P. Patel, J. Rochman, S. Meesala, W. Hong, Q. Quan, M. D. Lukin, and M. Lončar, Nat. Comm. **5**, 5718 (2014).
